# Supplementary material for: ExecHMR: Transition-Aware Recovery of Robot-Executable Human Motion with Bidirectional Alignment
Source: arXiv:2611.38651 source file (2026-11-28)
Supplement: Supplementary file 1 [file real_supp_tikz.tex]

% Supplementary real-robot deployments in the format of Fig. 6 (figures/real_robot.tex): per instant, the input frame,
% the camera-frame mesh of ExecHMR (s500k) over it (same crop) and the LimX Luna recording at the aligned instant (one
% constant offset per video from ViTPose limb directions). Tiles and pose similarities from
% paper_sa120/scripts/real3_assets.py (data/real3/fidelity_<clip>.json).
\definecolor{rrOurs}{RGB}{40,92,186}
% #1 clip letter (tiles figures/real_supp/<clip>_{in,mesh,robot}<n>.jpg), #2 {column/seconds/similarity,...}
\newcommand{\realsupp}[2]{%
\resizebox{\textwidth}{!}{%
\begin{tikzpicture}[x=1pt,y=1pt,font=\scriptsize]
\def\tw{48}\def\th{72.33}\def\tg{1.6}\def\rg{1.6}\def\bw{25}% tile (aspect 0.664 as Fig. 6), gaps, bar
\def\tile##1##2##3{%
  \begin{scope}
    \clip[rounded corners=1.5pt] (##1,##2) rectangle ++(\tw,\th);
    \node[anchor=south west,inner sep=0pt] at (##1,##2) {\includegraphics[width=\tw pt,height=\th pt]{##3}};
  \end{scope}
  \draw[rounded corners=1.5pt,draw=black!25,line width=0.3pt] (##1,##2) rectangle ++(\tw,\th);}%
\pgfmathsetmacro\ym{\th+\rg}\pgfmathsetmacro\yv{2*(\th+\rg)}%
\foreach \c/\t/\s in {#2}{
  \pgfmathsetmacro\tx{(\c-1)*(\tw+\tg)}
  \tile{\tx}{\yv}{figures/real_supp/#1_in\c.jpg}
  \tile{\tx}{\ym}{figures/real_supp/#1_mesh\c.jpg}
  \tile{\tx}{0}{figures/real_supp/#1_robot\c.jpg}
  \node[anchor=north west,inner sep=1pt,fill=black,fill opacity=0.55,text opacity=1,text=white,rounded corners=1pt,
        font=\fontsize{6.4}{7}\selectfont\bfseries] at (\tx+1.5,\yv+\th-1.5) {\t\,s};
  \fill[black!10,rounded corners=1.2pt] (\tx+1.5,-6.6) rectangle ++(\bw,3);
  \fill[rrOurs,rounded corners=1.2pt] (\tx+1.5,-6.6) rectangle ++(\bw*\s,3);
  \node[anchor=east,inner sep=0pt,text=rrOurs,font=\fontsize{7}{7.6}\selectfont\bfseries] at (\tx+\tw-0.8,-5.1) {\s};}
\end{tikzpicture}}}
