# Supplementary material for: ExecHMR: Transition-Aware Recovery of Robot-Executable Human Motion with Bidirectional Alignment
Source: arXiv:2611.38651 source file (2026-11-28)
Supplement: Supplementary file 2 [file supp_cases_tikz.tex]

% Supplementary cases in the format of the teaser (Fig. 1, figures/teaser_tikz.tex): per clip, video frames with the
% camera-frame mesh of ExecHMR (s500k), GENMO -> robot and ExecHMR robot mode, each robot frame rendered from the video
% camera's viewpoint relative to the person (paper_sa120/scripts/supp_cases_assets.sh; tiles: ffmpeg scale=360:480).
\definecolor{tsOurs}{RGB}{40,92,186}
\definecolor{tsBase}{RGB}{92,92,92}
\definecolor{tsFall}{RGB}{204,45,38}
\definecolor{tsOk}{RGB}{34,139,62}
% #1 tile prefix, #2 time axis {column/seconds,...}, #3 time at which the GENMO robot fell (last column shows it down)
\newcommand{\suppcase}[3]{%
\resizebox{\linewidth}{!}{%
\begin{tikzpicture}[x=1pt,y=1pt,font=\scriptsize,
  badge/.style={rounded corners=1.2pt,inner sep=1.2pt,text=white,font=\fontsize{5.2}{6}\selectfont\bfseries,anchor=south}]
\def\tw{42}\def\th{56}\def\tg{2}\def\rg{3.5}\def\xo{13}
\def\tile##1##2##3##4{%
  \pgfmathsetmacro\tx{\xo+(##1-1)*(\tw+\tg)}
  \begin{scope}
    \clip[rounded corners=1.6pt] (\tx,##2) rectangle ++(\tw,\th);
    \node[anchor=south west,inner sep=0pt] at (\tx,##2) {\includegraphics[width=\tw pt,height=\th pt]{##3}};
  \end{scope}
  \draw[rounded corners=1.6pt,##4] (\tx,##2) rectangle ++(\tw,\th);}
\pgfmathsetmacro\yv{2*(\th+\rg)}
\pgfmathsetmacro\yb{\th+\rg}
\pgfmathsetmacro\ya{\yv+\th+4}
\draw[black!35,line width=0.4pt,-{Latex[length=3pt,width=2.4pt]}] (\xo,\ya) -- (\xo+5*\tw+4*\tg+2,\ya);
\foreach \c/\t in {#2}{
  \pgfmathsetmacro\cx{\xo+(\c-1)*(\tw+\tg)+\tw/2}
  \draw[black!35,line width=0.4pt] (\cx,\ya-1.3) -- (\cx,\ya+1.3);
  \node[anchor=south,inner sep=1.2pt,text=black!70,font=\fontsize{5.6}{6.5}\selectfont] at (\cx,\ya+1.2) {\t\,s};}
\foreach \c in {1,...,5}{
  \tile{\c}{\yv}{#1v\c.jpg}{draw=black!25,line width=0.3pt}
  \tile{\c}{0}{#1o\c.jpg}{draw=black!18,line width=0.3pt}}
\foreach \c in {1,...,4}{\tile{\c}{\yb}{#1b\c.jpg}{draw=black!18,line width=0.3pt}}
\tile{5}{\yb}{#1b5.jpg}{draw=tsFall,line width=0.9pt}
\draw[rounded corners=1.6pt,draw=tsOk,line width=0.9pt] (\xo+4*\tw+4*\tg,0) rectangle ++(\tw,\th);
\node[badge,fill=tsFall] at (\xo+4*\tw+4*\tg+\tw/2,\yb+2.2) {\ding{55}\,fell at #3\,s};
\node[badge,fill=tsOk] at (\xo+4*\tw+4*\tg+\tw/2,2.2) {\ding{51}\,clip executed};
\node[rotate=90,align=center,font=\fontsize{6.2}{6.8}\selectfont,text=black!80] at (\xo/2-0.5,\yv+\th/2)
  {\textbf{Input video}\\[-0.2pt]+ our mesh};
\node[rotate=90,align=center,font=\fontsize{6.2}{6.8}\selectfont,text=tsBase] at (\xo/2-0.5,\yb+\th/2)
  {\textbf{GENMO}\\[-0.2pt]$\rightarrow$ robot};
\node[rotate=90,align=center,font=\fontsize{6.2}{6.8}\selectfont,text=tsOurs] at (\xo/2-0.5,\th/2)
  {\textbf{\method}\\[-0.2pt]robot mode};
\end{tikzpicture}}}
\begin{minipage}[t]{0.485\textwidth}\centering
\suppcase{figures/supp_cases/dance_}{1/0.5,2/2.0,3/3.5,4/5.0,5/7.2}{6.2}\\[1pt]
{\small (a) EMDB-1 P5\_42, dancing (0--10\,s)}
\end{minipage}\hfill
\begin{minipage}[t]{0.485\textwidth}\centering
\suppcase{figures/supp_cases/cross_}{1/1.0,2/3.0,3/5.0,4/7.0,5/9.3}{8.3}\\[1pt]
{\small (b) 3DPW downtown\_crossStreets\_00, crossing a street (0--10\,s)}
\end{minipage}\\[7pt]
\begin{minipage}[t]{0.485\textwidth}\centering
\suppcase{figures/supp_cases/rect_}{1/0.5,2/2.0,3/3.5,4/5.0,5/7.3}{6.3}\\[1pt]
{\small (c) EMDB-2 P9\_79, walking a rectangle (0--10\,s)}
\end{minipage}\hfill
\begin{minipage}[t]{0.485\textwidth}\centering
\suppcase{figures/supp_cases/park_}{1/0.5,2/2.0,3/3.5,4/5.0,5/7.3}{6.3}\\[1pt]
{\small (d) EMDB-2 P7\_61, walking in a park (20--30\,s)}
\end{minipage}
